# Supplementary material for: Structure and thermodynamics of two dimensional Yukawa liquids
Source: arXiv:2104.04811 ancillary file (2021-04-14)
Supplement: Supplementary file 1 [file supplementary_material_final.pdf]

**Structure and thermodynamics of two dimensional Yukawa liquids**
**Supplementary material**

F. Lucco Castello and P. Tolias
*Space and Plasma Physics, Royal Institute of Technology, Stockholm, SE-100 44, Sweden*

Supplementary material for the manuscript entitled "Structure and thermodynamics of two dimensional Yukawa liquids". Structural and thermodynamic properties obtained from molecular dynamics simulations performed with 4096 particles in the canonical NVT ensemble, time-step $\Delta\tau = 0.001d\sqrt{m/(k_BT)}$ and an interaction potential truncated at $r = 20d$ for $\kappa = 0.5$ and at $r = 10d$ for $\kappa > 0.5$. Here $m$ is the unitary particle mass, $k_B$ Boltzmann's constant, $T$ the temperature, $d = (\pi n)^{-1/2}$ the two dimensional Wigner-Seitz radius and $n$ the particle number density.

# Contents

**Tables 1a-1f**: Key figures of merit of the radial distribution function resulting from molecular dynamics simulations. Each table illustrates the results for one value of the screening parameter belonging to the set $\kappa = \{0.5, 1.0, 1.5, 2.0, 2.5, 3.0\}$.

**Tables 2a-2f**: Thermodynamic properties including excess internal energy, excess pressure and excess inverse isothermal compressibility extracted from molecular dynamics simulations. Each table illustrates the results for one value of the screening parameter belonging to the set $\kappa = \{0.5, 1.0, 1.5, 2.0, 2.5, 3.0\}$.

**Table 1a.** Key figures of merit of the radial distribution function resulting from molecular dynamics simulations: the location of the edge of the correlation void approximated as $\arg_r\{g(r) = 0.5\}$, ($x_{\rm cv}$), the magnitude and location of the first maximum ($g_{\rm max1}$ and $x_{\rm max1}$), the magnitude and location of the first non-zero minimum ($g_{\rm min1}$ and $x_{\rm min1}$) and the magnitude and location of the second maximum ($g_{\rm max2}$ and $x_{\rm max2}$) . Here $x = r/d$ and $d$ is the Wigner-Seitz radius in two dimensions. **Results for $\boldsymbol{\kappa = 0.5}$.**

| $\Gamma$ | $\Gamma/\Gamma_{\rm m}$ | $x_{\rm cv}$ | $g_{\rm max1}$ | $x_{\rm max1}$ | $g_{\rm min1}$ | $x_{\rm min1}$ | $g_{\rm max2}$ | $x_{\rm max2}$ |
|---|---|---|---|---|---|---|---|---|
| 15.0 | 0.11 | 1.095 | 1.181 | 1.669 | 0.962 | 2.581 | 1.010 | 3.483 |
| 20.0 | 0.14 | 1.115 | 1.214 | 1.687 | 0.951 | 2.605 | 1.012 | 3.511 |
| 25.0 | 0.18 | 1.135 | 1.243 | 1.693 | 0.937 | 2.579 | 1.018 | 3.495 |
| 30.0 | 0.21 | 1.207 | 1.384 | 1.719 | 0.877 | 2.613 | 1.045 | 3.469 |
| 35.0 | 0.25 | 1.255 | 1.506 | 1.717 | 0.824 | 2.615 | 1.075 | 3.455 |
| 40.0 | 0.28 | 1.289 | 1.613 | 1.737 | 0.772 | 2.627 | 1.111 | 3.467 |
| 45.0 | 0.32 | 1.319 | 1.715 | 1.757 | 0.729 | 2.623 | 1.143 | 3.473 |
| 50.0 | 0.35 | 1.341 | 1.808 | 1.745 | 0.689 | 2.643 | 1.175 | 3.489 |
| 55.0 | 0.39 | 1.361 | 1.894 | 1.773 | 0.657 | 2.645 | 1.207 | 3.475 |
| 60.0 | 0.42 | 1.377 | 1.975 | 1.767 | 0.627 | 2.651 | 1.239 | 3.503 |
| 65.0 | 0.46 | 1.393 | 2.048 | 1.779 | 0.600 | 2.629 | 1.272 | 3.501 |
| 70.0 | 0.49 | 1.407 | 2.121 | 1.783 | 0.575 | 2.659 | 1.299 | 3.509 |
| 75.0 | 0.53 | 1.419 | 2.192 | 1.785 | 0.553 | 2.649 | 1.328 | 3.503 |
| 80.0 | 0.56 | 1.429 | 2.255 | 1.789 | 0.537 | 2.633 | 1.355 | 3.509 |
| 85.0 | 0.60 | 1.439 | 2.320 | 1.781 | 0.516 | 2.643 | 1.383 | 3.511 |
| 90.0 | 0.63 | 1.449 | 2.385 | 1.793 | 0.499 | 2.625 | 1.406 | 3.505 |
| 95.0 | 0.67 | 1.457 | 2.443 | 1.789 | 0.483 | 2.643 | 1.429 | 3.525 |
| 100.0 | 0.70 | 1.465 | 2.501 | 1.795 | 0.468 | 2.645 | 1.449 | 3.499 |
| 105.0 | 0.74 | 1.473 | 2.558 | 1.791 | 0.452 | 2.651 | 1.475 | 3.517 |
| 110.0 | 0.77 | 1.479 | 2.616 | 1.807 | 0.440 | 2.625 | 1.495 | 3.525 |
| 115.0 | 0.81 | 1.485 | 2.670 | 1.811 | 0.426 | 2.617 | 1.511 | 3.527 |
| 120.0 | 0.84 | 1.491 | 2.722 | 1.803 | 0.414 | 2.645 | 1.533 | 3.509 |
| 125.0 | 0.88 | 1.497 | 2.773 | 1.803 | 0.400 | 2.635 | 1.551 | 3.531 |
| 130.0 | 0.91 | 1.503 | 2.826 | 1.805 | 0.383 | 2.613 | 1.570 | 3.531 |
| 135.0 | 0.95 | 1.509 | 2.877 | 1.809 | 0.369 | 2.617 | 1.583 | 3.537 |

**Table 1b.** Key figures of merit of the radial distribution function resulting from molecular dynamics simulations: the location of the edge of the correlation void approximated as $\arg_r\{g(r) = 0.5\}$, ($x_{\rm cv}$), the magnitude and location of the first maximum ($g_{\rm max1}$ and $x_{\rm max1}$), the magnitude and location of the first non-zero minimum ($g_{\rm min1}$ and $x_{\rm min1}$) and the magnitude and location of the second maximum ($g_{\rm max2}$ and $x_{\rm max2}$) . Here $x = r/d$ and $d$ is the Wigner-Seitz radius in two dimensions. **Results for $\boldsymbol{\kappa} = \mathbf{1.0}$.**

| $\Gamma$ | $\Gamma/\Gamma_{\rm m}$ | $x_{\rm cv}$ | $g_{\rm max1}$ | $x_{\rm max1}$ | $g_{\rm min1}$ | $x_{\rm min1}$ | $g_{\rm max2}$ | $x_{\rm max2}$ |
|---|---|---|---|---|---|---|---|---|
| 20.0 | 0.11 | 1.085 | 1.189 | 1.649 | 0.961 | 2.525 | 1.008 | 3.409 |
| 25.0 | 0.14 | 1.159 | 1.308 | 1.691 | 0.916 | 2.583 | 1.024 | 3.453 |
| 30.0 | 0.17 | 1.211 | 1.414 | 1.699 | 0.868 | 2.577 | 1.047 | 3.473 |
| 35.0 | 0.20 | 1.247 | 1.508 | 1.717 | 0.824 | 2.567 | 1.074 | 3.483 |
| 40.0 | 0.22 | 1.277 | 1.594 | 1.731 | 0.787 | 2.591 | 1.101 | 3.465 |
| 45.0 | 0.25 | 1.303 | 1.673 | 1.723 | 0.750 | 2.625 | 1.125 | 3.461 |
| 50.0 | 0.28 | 1.323 | 1.748 | 1.733 | 0.716 | 2.605 | 1.153 | 3.491 |
| 55.0 | 0.31 | 1.341 | 1.819 | 1.757 | 0.686 | 2.629 | 1.178 | 3.481 |
| 60.0 | 0.34 | 1.357 | 1.886 | 1.761 | 0.659 | 2.621 | 1.204 | 3.483 |
| 65.0 | 0.37 | 1.371 | 1.950 | 1.753 | 0.637 | 2.645 | 1.230 | 3.489 |
| 70.0 | 0.39 | 1.383 | 2.014 | 1.765 | 0.613 | 2.645 | 1.252 | 3.517 |
| 75.0 | 0.42 | 1.395 | 2.069 | 1.763 | 0.593 | 2.643 | 1.276 | 3.483 |
| 80.0 | 0.45 | 1.405 | 2.128 | 1.779 | 0.574 | 2.649 | 1.300 | 3.481 |
| 85.0 | 0.48 | 1.415 | 2.182 | 1.779 | 0.556 | 2.627 | 1.323 | 3.483 |
| 90.0 | 0.51 | 1.423 | 2.235 | 1.783 | 0.539 | 2.649 | 1.344 | 3.507 |
| 95.0 | 0.53 | 1.431 | 2.287 | 1.781 | 0.525 | 2.649 | 1.364 | 3.513 |
| 100.0 | 0.56 | 1.439 | 2.335 | 1.787 | 0.511 | 2.645 | 1.386 | 3.495 |
| 105.0 | 0.59 | 1.447 | 2.384 | 1.787 | 0.496 | 2.637 | 1.402 | 3.495 |
| 110.0 | 0.62 | 1.453 | 2.433 | 1.783 | 0.483 | 2.627 | 1.423 | 3.503 |
| 115.0 | 0.65 | 1.461 | 2.479 | 1.793 | 0.471 | 2.619 | 1.440 | 3.503 |
| 120.0 | 0.67 | 1.467 | 2.527 | 1.795 | 0.460 | 2.643 | 1.458 | 3.515 |
| 125.0 | 0.70 | 1.473 | 2.569 | 1.799 | 0.449 | 2.629 | 1.475 | 3.513 |
| 130.0 | 0.73 | 1.477 | 2.613 | 1.799 | 0.437 | 2.631 | 1.493 | 3.513 |
| 135.0 | 0.76 | 1.483 | 2.656 | 1.797 | 0.425 | 2.625 | 1.509 | 3.513 |
| 140.0 | 0.79 | 1.487 | 2.697 | 1.811 | 0.414 | 2.623 | 1.523 | 3.527 |
| 145.0 | 0.81 | 1.493 | 2.741 | 1.813 | 0.404 | 2.609 | 1.538 | 3.523 |
| 150.0 | 0.84 | 1.497 | 2.781 | 1.805 | 0.393 | 2.623 | 1.551 | 3.527 |
| 155.0 | 0.87 | 1.501 | 2.822 | 1.813 | 0.382 | 2.635 | 1.563 | 3.527 |
| 160.0 | 0.90 | 1.507 | 2.864 | 1.815 | 0.370 | 2.623 | 1.576 | 3.513 |
| 165.0 | 0.93 | 1.511 | 2.907 | 1.815 | 0.359 | 2.617 | 1.591 | 3.529 |

**Table 1c.** Key figures of merit of the radial distribution function resulting from molecular dynamics simulations: the location of the edge of the correlation void approximated as $\arg_r\{g(r) = 0.5\}$, ($x_{\rm cv}$), the magnitude and location of the first maximum ($g_{\rm max1}$ and $x_{\rm max1}$), the magnitude and location of the first non-zero minimum ($g_{\rm min1}$ and $x_{\rm min1}$) and the magnitude and location of the second maximum ($g_{\rm max2}$ and $x_{\rm max2}$) . Here $x = r/d$ and $d$ is the Wigner-Seitz radius in two dimensions. **Results for $\boldsymbol{\kappa} = \mathbf{1.5}$**.

| $\Gamma$ | $\Gamma/\Gamma_{\rm m}$ | $x_{\rm cv}$ | $g_{\rm max1}$ | $x_{\rm max1}$ | $g_{\rm min1}$ | $x_{\rm min1}$ | $g_{\rm max2}$ | $x_{\rm max2}$ |
|---|---|---|---|---|---|---|---|---|
| 30.0 | 0.12 | 1.015 | 1.135 | 1.597 | 0.980 | 2.525 | 1.003 | 3.523 |
| 40.0 | 0.16 | 1.145 | 1.307 | 1.641 | 0.919 | 2.533 | 1.022 | 3.371 |
| 50.0 | 0.20 | 1.217 | 1.451 | 1.681 | 0.856 | 2.551 | 1.055 | 3.431 |
| 60.0 | 0.24 | 1.265 | 1.576 | 1.689 | 0.798 | 2.597 | 1.091 | 3.439 |
| 70.0 | 0.28 | 1.301 | 1.688 | 1.725 | 0.746 | 2.599 | 1.126 | 3.469 |
| 80.0 | 0.32 | 1.329 | 1.790 | 1.725 | 0.702 | 2.605 | 1.165 | 3.463 |
| 90.0 | 0.36 | 1.353 | 1.886 | 1.751 | 0.663 | 2.623 | 1.200 | 3.467 |
| 100.0 | 0.40 | 1.371 | 1.974 | 1.739 | 0.631 | 2.629 | 1.235 | 3.465 |
| 110.0 | 0.44 | 1.389 | 2.058 | 1.765 | 0.599 | 2.627 | 1.269 | 3.487 |
| 120.0 | 0.48 | 1.405 | 2.137 | 1.763 | 0.575 | 2.649 | 1.300 | 3.491 |
| 130.0 | 0.52 | 1.417 | 2.210 | 1.773 | 0.548 | 2.643 | 1.330 | 3.491 |
| 140.0 | 0.56 | 1.429 | 2.283 | 1.763 | 0.527 | 2.639 | 1.360 | 3.475 |
| 150.0 | 0.60 | 1.441 | 2.355 | 1.783 | 0.506 | 2.643 | 1.388 | 3.481 |
| 160.0 | 0.64 | 1.451 | 2.419 | 1.783 | 0.488 | 2.641 | 1.413 | 3.507 |
| 170.0 | 0.68 | 1.459 | 2.485 | 1.783 | 0.469 | 2.637 | 1.439 | 3.497 |
| 180.0 | 0.72 | 1.467 | 2.548 | 1.789 | 0.454 | 2.625 | 1.464 | 3.497 |
| 190.0 | 0.76 | 1.477 | 2.608 | 1.797 | 0.437 | 2.637 | 1.487 | 3.507 |
| 200.0 | 0.80 | 1.483 | 2.670 | 1.803 | 0.421 | 2.629 | 1.508 | 3.505 |
| 210.0 | 0.84 | 1.491 | 2.728 | 1.791 | 0.406 | 2.625 | 1.529 | 3.513 |
| 220.0 | 0.88 | 1.497 | 2.787 | 1.805 | 0.390 | 2.629 | 1.549 | 3.513 |
| 230.0 | 0.92 | 1.503 | 2.844 | 1.807 | 0.374 | 2.617 | 1.569 | 3.511 |

**Table 1d.** Key figures of merit of the radial distribution function resulting from molecular dynamics simulations: the location of the edge of the correlation void approximated as $\arg_r\{g(r) = 0.5\}$, ($x_{\rm cv}$), the magnitude and location of the first maximum ($g_{\rm max1}$ and $x_{\rm max1}$), the magnitude and location of the first non-zero minimum ($g_{\rm min1}$ and $x_{\rm min1}$) and the magnitude and location of the second maximum ($g_{\rm max2}$ and $x_{\rm max2}$) . Here $x = r/d$ and $d$ is the Wigner-Seitz radius in two dimensions. **Results for $\boldsymbol{\kappa} = \mathbf{2.0}$**.

| $\Gamma$ | $\Gamma/\Gamma_{\rm m}$ | $x_{\rm cv}$ | $g_{\rm max1}$ | $x_{\rm max1}$ | $g_{\rm min1}$ | $x_{\rm min1}$ | $g_{\rm max2}$ | $x_{\rm max2}$ |
|---|---|---|---|---|---|---|---|---|
| 45.0 | 0.11 | 1.015 | 1.157 | 1.537 | 0.975 | 2.413 | 1.004 | 3.259 |
| 60.0 | 0.15 | 1.141 | 1.325 | 1.607 | 0.916 | 2.489 | 1.023 | 3.443 |
| 75.0 | 0.19 | 1.211 | 1.465 | 1.661 | 0.856 | 2.549 | 1.055 | 3.345 |
| 90.0 | 0.23 | 1.259 | 1.582 | 1.691 | 0.799 | 2.557 | 1.088 | 3.385 |
| 105.0 | 0.27 | 1.295 | 1.692 | 1.695 | 0.749 | 2.589 | 1.122 | 3.407 |
| 120.0 | 0.30 | 1.323 | 1.788 | 1.719 | 0.708 | 2.589 | 1.158 | 3.435 |
| 135.0 | 0.34 | 1.347 | 1.880 | 1.729 | 0.671 | 2.613 | 1.192 | 3.445 |
| 150.0 | 0.38 | 1.367 | 1.964 | 1.731 | 0.639 | 2.607 | 1.224 | 3.445 |
| 165.0 | 0.42 | 1.383 | 2.043 | 1.745 | 0.609 | 2.605 | 1.257 | 3.469 |
| 180.0 | 0.46 | 1.399 | 2.121 | 1.747 | 0.583 | 2.633 | 1.286 | 3.463 |
| 195.0 | 0.49 | 1.411 | 2.195 | 1.761 | 0.558 | 2.627 | 1.316 | 3.469 |
| 210.0 | 0.53 | 1.423 | 2.263 | 1.769 | 0.538 | 2.641 | 1.344 | 3.463 |
| 225.0 | 0.57 | 1.435 | 2.331 | 1.767 | 0.517 | 2.617 | 1.374 | 3.479 |
| 240.0 | 0.61 | 1.445 | 2.395 | 1.771 | 0.498 | 2.647 | 1.399 | 3.491 |
| 255.0 | 0.64 | 1.453 | 2.456 | 1.775 | 0.479 | 2.633 | 1.424 | 3.487 |
| 270.0 | 0.68 | 1.463 | 2.519 | 1.787 | 0.463 | 2.613 | 1.445 | 3.501 |
| 285.0 | 0.72 | 1.471 | 2.578 | 1.779 | 0.447 | 2.625 | 1.469 | 3.495 |
| 300.0 | 0.76 | 1.477 | 2.633 | 1.779 | 0.431 | 2.625 | 1.490 | 3.499 |
| 315.0 | 0.80 | 1.485 | 2.695 | 1.787 | 0.416 | 2.605 | 1.511 | 3.515 |
| 330.0 | 0.83 | 1.491 | 2.750 | 1.797 | 0.400 | 2.609 | 1.529 | 3.515 |
| 345.0 | 0.87 | 1.497 | 2.804 | 1.791 | 0.386 | 2.601 | 1.548 | 3.507 |
| 360.0 | 0.91 | 1.503 | 2.859 | 1.801 | 0.371 | 2.621 | 1.566 | 3.503 |
| 375.0 | 0.95 | 1.509 | 2.917 | 1.799 | 0.354 | 2.607 | 1.583 | 3.505 |

**Table 1e.** Key figures of merit of the radial distribution function resulting from molecular dynamics simulations: the location of the edge of the correlation void approximated as $\arg_r\{g(r) = 0.5\}$, ($x_{\rm cv}$), the magnitude and location of the first maximum ($g_{\rm max1}$ and $x_{\rm max1}$), the magnitude and location of the first non-zero minimum ($g_{\rm min1}$ and $x_{\rm min1}$) and the magnitude and location of the second maximum ($g_{\rm max2}$ and $x_{\rm max2}$) . Here $x = r/d$ and $d$ is the Wigner-Seitz radius in two dimensions. **Results for $\boldsymbol{\kappa = 2.5}$**.

| $\Gamma$ | $\Gamma/\Gamma_{\rm m}$ | $x_{\rm cv}$ | $g_{\rm max1}$ | $x_{\rm max1}$ | $g_{\rm min1}$ | $x_{\rm min1}$ | $g_{\rm max2}$ | $x_{\rm max2}$ |
|---|---|---|---|---|---|---|---|---|
| 80.0 | 0.12 | 1.111 | 1.301 | 1.583 | 0.929 | 2.395 | 1.019 | 3.279 |
| 100.0 | 0.15 | 1.181 | 1.418 | 1.627 | 0.878 | 2.501 | 1.042 | 3.289 |
| 120.0 | 0.18 | 1.227 | 1.523 | 1.641 | 0.832 | 2.515 | 1.068 | 3.369 |
| 140.0 | 0.21 | 1.263 | 1.616 | 1.667 | 0.790 | 2.527 | 1.095 | 3.373 |
| 160.0 | 0.23 | 1.291 | 1.701 | 1.695 | 0.752 | 2.563 | 1.122 | 3.385 |
| 180.0 | 0.26 | 1.315 | 1.780 | 1.691 | 0.719 | 2.585 | 1.149 | 3.403 |
| 200.0 | 0.29 | 1.335 | 1.855 | 1.705 | 0.689 | 2.565 | 1.175 | 3.427 |
| 220.0 | 0.32 | 1.351 | 1.921 | 1.723 | 0.660 | 2.605 | 1.201 | 3.413 |
| 240.0 | 0.35 | 1.367 | 1.988 | 1.717 | 0.636 | 2.595 | 1.227 | 3.443 |
| 260.0 | 0.38 | 1.381 | 2.052 | 1.731 | 0.613 | 2.605 | 1.252 | 3.417 |
| 280.0 | 0.41 | 1.393 | 2.113 | 1.735 | 0.592 | 2.611 | 1.277 | 3.449 |
| 300.0 | 0.44 | 1.405 | 2.171 | 1.743 | 0.574 | 2.627 | 1.302 | 3.457 |
| 320.0 | 0.47 | 1.415 | 2.227 | 1.745 | 0.554 | 2.621 | 1.321 | 3.443 |
| 340.0 | 0.50 | 1.425 | 2.283 | 1.753 | 0.537 | 2.629 | 1.346 | 3.459 |
| 360.0 | 0.53 | 1.433 | 2.337 | 1.767 | 0.521 | 2.637 | 1.367 | 3.467 |
| 380.0 | 0.56 | 1.441 | 2.385 | 1.761 | 0.506 | 2.627 | 1.389 | 3.467 |
| 400.0 | 0.59 | 1.449 | 2.436 | 1.761 | 0.492 | 2.613 | 1.408 | 3.473 |
| 420.0 | 0.62 | 1.455 | 2.484 | 1.767 | 0.478 | 2.619 | 1.424 | 3.473 |
| 440.0 | 0.65 | 1.463 | 2.532 | 1.771 | 0.465 | 2.625 | 1.445 | 3.477 |
| 460.0 | 0.67 | 1.469 | 2.577 | 1.769 | 0.452 | 2.627 | 1.463 | 3.481 |
| 480.0 | 0.70 | 1.475 | 2.622 | 1.779 | 0.439 | 2.615 | 1.478 | 3.505 |
| 500.0 | 0.73 | 1.481 | 2.669 | 1.779 | 0.427 | 2.623 | 1.494 | 3.489 |
| 520.0 | 0.76 | 1.485 | 2.713 | 1.785 | 0.414 | 2.615 | 1.509 | 3.507 |
| 540.0 | 0.79 | 1.491 | 2.758 | 1.781 | 0.403 | 2.619 | 1.526 | 3.489 |
| 560.0 | 0.82 | 1.497 | 2.800 | 1.793 | 0.392 | 2.615 | 1.538 | 3.487 |
| 580.0 | 0.85 | 1.501 | 2.843 | 1.789 | 0.380 | 2.613 | 1.554 | 3.483 |
| 600.0 | 0.88 | 1.505 | 2.888 | 1.787 | 0.367 | 2.609 | 1.568 | 3.505 |
| 620.0 | 0.91 | 1.511 | 2.929 | 1.801 | 0.353 | 2.609 | 1.583 | 3.505 |
| 640.0 | 0.94 | 1.515 | 2.974 | 1.797 | 0.340 | 2.613 | 1.595 | 3.507 |

**Table 1f.** Key figures of merit of the radial distribution function resulting from molecular dynamics simulations: the location of the edge of the correlation void approximated as $\arg_r\{g(r) = 0.5\}$, ($x_{\rm cv}$), the magnitude and location of the first maximum ($g_{\rm max1}$ and $x_{\rm max1}$), the magnitude and location of the first non-zero minimum ($g_{\rm min1}$ and $x_{\rm min1}$) and the magnitude and location of the second maximum ($g_{\rm max2}$ and $x_{\rm max2}$) . Here $x = r/d$ and $d$ is the Wigner-Seitz radius in two dimensions. **Results for $\boldsymbol{\kappa} = \mathbf{3.0}$.**

| $\Gamma$ | $\Gamma/\Gamma_{\rm m}$ | $x_{\rm cv}$ | $g_{\rm max1}$ | $x_{\rm max1}$ | $g_{\rm min1}$ | $x_{\rm min1}$ | $g_{\rm max2}$ | $x_{\rm max2}$ |
|---|---|---|---|---|---|---|---|---|
| 150.0 | 0.13 | 1.069 | 1.262 | 1.517 | 0.945 | 2.365 | 1.013 | 3.167 |
| 200.0 | 0.18 | 1.181 | 1.445 | 1.581 | 0.872 | 2.443 | 1.045 | 3.315 |
| 250.0 | 0.22 | 1.245 | 1.589 | 1.639 | 0.808 | 2.515 | 1.084 | 3.307 |
| 300.0 | 0.27 | 1.289 | 1.712 | 1.673 | 0.752 | 2.561 | 1.120 | 3.377 |
| 350.0 | 0.31 | 1.321 | 1.824 | 1.679 | 0.706 | 2.571 | 1.159 | 3.369 |
| 400.0 | 0.35 | 1.347 | 1.924 | 1.713 | 0.668 | 2.571 | 1.195 | 3.417 |
| 450.0 | 0.40 | 1.369 | 2.019 | 1.713 | 0.633 | 2.603 | 1.230 | 3.433 |
| 500.0 | 0.44 | 1.389 | 2.103 | 1.725 | 0.604 | 2.599 | 1.266 | 3.435 |
| 550.0 | 0.49 | 1.405 | 2.186 | 1.741 | 0.575 | 2.607 | 1.300 | 3.439 |
| 600.0 | 0.53 | 1.419 | 2.265 | 1.747 | 0.551 | 2.613 | 1.331 | 3.445 |
| 650.0 | 0.58 | 1.431 | 2.339 | 1.735 | 0.527 | 2.621 | 1.359 | 3.461 |
| 700.0 | 0.62 | 1.443 | 2.412 | 1.753 | 0.506 | 2.627 | 1.389 | 3.455 |
| 750.0 | 0.67 | 1.453 | 2.478 | 1.765 | 0.487 | 2.605 | 1.414 | 3.459 |
| 800.0 | 0.71 | 1.463 | 2.546 | 1.761 | 0.468 | 2.609 | 1.440 | 3.457 |
| 850.0 | 0.75 | 1.471 | 2.609 | 1.771 | 0.451 | 2.619 | 1.466 | 3.463 |
| 900.0 | 0.80 | 1.479 | 2.673 | 1.771 | 0.433 | 2.615 | 1.489 | 3.471 |
| 950.0 | 0.84 | 1.487 | 2.734 | 1.781 | 0.416 | 2.619 | 1.512 | 3.495 |
| 1000.0 | 0.89 | 1.495 | 2.795 | 1.787 | 0.400 | 2.619 | 1.530 | 3.495 |
| 1050.0 | 0.93 | 1.501 | 2.853 | 1.781 | 0.382 | 2.607 | 1.552 | 3.491 |

**Table 2a.** Reduced excess internal energy, $u_{\mathrm{ex}}$, reduced excess pressure, $p_{\mathrm{ex}}$, and reduced excess inverse isothermal compressibility, $\mu_{\mathrm{ex}}$, resulting from molecular dynamics simulations. The standard deviation of the internal energy, $\sigma[u_{\mathrm{ex}}]$, and the standard deviation of the pressure, $\sigma[p_{\mathrm{ex}}]$, were estimated directly from the fluctuations sampled during the course of the simulation, while the standard deviation of the inverse isothermal compressibility, $\sigma[\mu_{\mathrm{ex}}]$, was estimated with the bootstrap resampling technique. **Results for $\boldsymbol{\kappa} = \mathbf{0.5}$.**

| $\Gamma$ | $\Gamma/\Gamma_{\mathrm{m}}$ | $u_{\mathrm{ex}}$ | $\sigma[u_{\mathrm{ex}}] \times 10^3$ | $p_{\mathrm{ex}}$ | $\sigma[p_{\mathrm{ex}}] \times 10^3$ | $\mu_{\mathrm{ex}}$ | $\sigma[\mu_{\mathrm{ex}}] \times 10^3$ |
|---|---|---|---|---|---|---|---|
| 15.0 | 0.11 | 17.602 | 0.272 | 22.384 | 0.173 | 32.216 | 0.146 |
| 20.0 | 0.14 | 23.262 | 0.275 | 29.716 | 0.176 | 48.128 | 0.167 |
| 25.0 | 0.18 | 28.911 | 0.288 | 37.039 | 0.181 | 64.056 | 0.182 |
| 30.0 | 0.21 | 34.550 | 0.293 | 44.358 | 0.186 | 79.961 | 0.187 |
| 35.0 | 0.25 | 40.184 | 0.300 | 51.674 | 0.188 | 95.863 | 0.219 |
| 40.0 | 0.28 | 45.814 | 0.309 | 58.987 | 0.194 | 111.767 | 0.210 |
| 45.0 | 0.32 | 51.438 | 0.308 | 66.297 | 0.192 | 127.658 | 0.215 |
| 50.0 | 0.35 | 57.061 | 0.322 | 73.606 | 0.201 | 143.565 | 0.212 |
| 55.0 | 0.39 | 62.681 | 0.330 | 80.914 | 0.207 | 159.438 | 0.240 |
| 60.0 | 0.42 | 68.300 | 0.330 | 88.220 | 0.205 | 175.319 | 0.261 |
| 65.0 | 0.46 | 73.916 | 0.337 | 95.525 | 0.210 | 191.223 | 0.232 |
| 70.0 | 0.49 | 79.530 | 0.337 | 102.829 | 0.209 | 207.103 | 0.242 |
| 75.0 | 0.53 | 85.145 | 0.338 | 110.133 | 0.209 | 222.999 | 0.256 |
| 80.0 | 0.56 | 90.757 | 0.342 | 117.436 | 0.211 | 238.893 | 0.242 |
| 85.0 | 0.60 | 96.368 | 0.334 | 124.738 | 0.208 | 254.778 | 0.269 |
| 90.0 | 0.63 | 101.978 | 0.344 | 132.040 | 0.214 | 270.683 | 0.255 |
| 95.0 | 0.67 | 107.588 | 0.358 | 139.341 | 0.222 | 286.553 | 0.262 |
| 100.0 | 0.70 | 113.197 | 0.350 | 146.641 | 0.217 | 302.413 | 0.292 |
| 105.0 | 0.74 | 118.804 | 0.364 | 153.942 | 0.223 | 318.322 | 0.265 |
| 110.0 | 0.77 | 124.411 | 0.365 | 161.240 | 0.224 | 334.186 | 0.276 |
| 115.0 | 0.81 | 130.015 | 0.370 | 168.539 | 0.227 | 350.073 | 0.275 |
| 120.0 | 0.84 | 135.618 | 0.365 | 175.836 | 0.225 | 365.948 | 0.299 |
| 125.0 | 0.88 | 141.221 | 0.388 | 183.134 | 0.238 | 381.841 | 0.288 |
| 130.0 | 0.91 | 146.821 | 0.407 | 190.430 | 0.249 | 397.673 | 0.306 |
| 135.0 | 0.95 | 152.417 | 0.411 | 197.723 | 0.251 | 413.512 | 0.370 |

**Table 2b.** Reduced excess internal energy, $u_{\mathrm{ex}}$, reduced excess pressure, $p_{\mathrm{ex}}$, and reduced excess inverse isothermal compressibility, $\mu_{\mathrm{ex}}$, resulting from molecular dynamics simulations. The standard deviation of the internal energy, $\sigma[u_{\mathrm{ex}}]$, and the standard deviation of the pressure, $\sigma[p_{\mathrm{ex}}]$, were estimated directly from the fluctuations sampled during the course of the simulation, while the standard deviation of the inverse isothermal compressibility, $\sigma[\mu_{\mathrm{ex}}]$, was estimated with the bootstrap resampling technique. **Results for $\boldsymbol{\kappa = 1.0}$.**

| $\Gamma$ | $\Gamma/\Gamma_{\mathrm{m}}$ | $u_{\mathrm{ex}}$ | $\sigma[u_{\mathrm{ex}}] \times 10^3$ | $p_{\mathrm{ex}}$ | $\sigma[p_{\mathrm{ex}}] \times 10^3$ | $\mu_{\mathrm{ex}}$ | $\sigma[\mu_{\mathrm{ex}}] \times 10^3$ |
|---|---|---|---|---|---|---|---|
| 20.0 | 0.11 | 6.761 | 0.265 | 10.549 | 0.231 | 24.580 | 0.308 |
| 25.0 | 0.14 | 8.298 | 0.270 | 13.054 | 0.239 | 30.599 | 0.325 |
| 30.0 | 0.17 | 9.828 | 0.287 | 15.552 | 0.250 | 36.591 | 0.372 |
| 35.0 | 0.20 | 11.350 | 0.293 | 18.044 | 0.257 | 42.589 | 0.379 |
| 40.0 | 0.22 | 12.871 | 0.295 | 20.535 | 0.258 | 48.612 | 0.353 |
| 45.0 | 0.25 | 14.386 | 0.300 | 23.020 | 0.262 | 54.614 | 0.403 |
| 50.0 | 0.28 | 15.899 | 0.305 | 25.504 | 0.269 | 60.601 | 0.417 |
| 55.0 | 0.31 | 17.408 | 0.306 | 27.985 | 0.268 | 66.617 | 0.406 |
| 60.0 | 0.34 | 18.917 | 0.308 | 30.465 | 0.270 | 72.617 | 0.450 |
| 65.0 | 0.37 | 20.422 | 0.316 | 32.943 | 0.275 | 78.602 | 0.425 |
| 70.0 | 0.39 | 21.928 | 0.316 | 35.421 | 0.277 | 84.602 | 0.434 |
| 75.0 | 0.42 | 23.431 | 0.326 | 37.896 | 0.285 | 90.568 | 0.465 |
| 80.0 | 0.45 | 24.933 | 0.330 | 40.370 | 0.288 | 96.550 | 0.477 |
| 85.0 | 0.48 | 26.437 | 0.331 | 42.847 | 0.288 | 102.560 | 0.498 |
| 90.0 | 0.51 | 27.937 | 0.323 | 45.319 | 0.280 | 108.598 | 0.427 |
| 95.0 | 0.53 | 29.437 | 0.338 | 47.792 | 0.294 | 114.532 | 0.522 |
| 100.0 | 0.56 | 30.935 | 0.328 | 50.264 | 0.286 | 120.570 | 0.483 |
| 105.0 | 0.59 | 32.434 | 0.333 | 52.736 | 0.289 | 126.552 | 0.507 |
| 110.0 | 0.62 | 33.934 | 0.337 | 55.208 | 0.294 | 132.530 | 0.485 |
| 115.0 | 0.65 | 35.430 | 0.345 | 57.678 | 0.301 | 138.491 | 0.531 |
| 120.0 | 0.67 | 36.926 | 0.354 | 60.148 | 0.306 | 144.461 | 0.505 |
| 125.0 | 0.70 | 38.421 | 0.348 | 62.617 | 0.302 | 150.476 | 0.534 |
| 130.0 | 0.73 | 39.917 | 0.351 | 65.086 | 0.304 | 156.463 | 0.542 |
| 135.0 | 0.76 | 41.412 | 0.359 | 67.555 | 0.309 | 162.429 | 0.599 |
| 140.0 | 0.79 | 42.904 | 0.359 | 70.022 | 0.310 | 168.417 | 0.568 |
| 145.0 | 0.81 | 44.399 | 0.360 | 72.491 | 0.311 | 174.407 | 0.565 |
| 150.0 | 0.84 | 45.891 | 0.373 | 74.957 | 0.320 | 180.347 | 0.610 |
| 155.0 | 0.87 | 47.381 | 0.370 | 77.422 | 0.318 | 186.348 | 0.564 |
| 160.0 | 0.90 | 48.872 | 0.395 | 79.887 | 0.337 | 192.238 | 0.645 |
| 165.0 | 0.93 | 50.357 | 0.389 | 82.348 | 0.332 | 198.245 | 0.634 |

**Table 2c.** Reduced excess internal energy, $u_{\rm ex}$, reduced excess pressure, $p_{\rm ex}$, and reduced excess inverse isothermal compressibility, $\mu_{\rm ex}$, resulting from molecular dynamics simulations. The standard deviation of the internal energy, $\sigma[u_{\rm ex}]$, and the standard deviation of the pressure, $\sigma[p_{\rm ex}]$, were estimated directly from the fluctuations sampled during the course of the simulation, while the standard deviation of the inverse isothermal compressibility, $\sigma[\mu_{\rm ex}]$, was estimated with the bootstrap resampling technique. **Results for $\boldsymbol{\kappa} = \mathbf{1.5}$.**

| $\Gamma$ | $\Gamma/\Gamma_{\rm m}$ | $u_{\rm ex}$ | $\sigma[u_{\rm ex}] \times 10^3$ | $p_{\rm ex}$ | $\sigma[p_{\rm ex}] \times 10^3$ | $\mu_{\rm ex}$ | $\sigma[\mu_{\rm ex}] \times 10^3$ |
|---|---|---|---|---|---|---|---|
| 30.0 | 0.12 | 3.828 | 0.261 | 7.129 | 0.302 | 17.910 | 0.546 |
| 40.0 | 0.16 | 4.902 | 0.278 | 9.273 | 0.323 | 23.615 | 0.614 |
| 50.0 | 0.20 | 5.962 | 0.288 | 11.400 | 0.339 | 29.299 | 0.665 |
| 60.0 | 0.24 | 7.012 | 0.282 | 13.514 | 0.333 | 35.092 | 0.625 |
| 70.0 | 0.28 | 8.057 | 0.296 | 15.621 | 0.351 | 40.734 | 0.711 |
| 80.0 | 0.32 | 9.094 | 0.301 | 17.720 | 0.359 | 46.424 | 0.771 |
| 90.0 | 0.36 | 10.131 | 0.309 | 19.818 | 0.366 | 52.111 | 0.780 |
| 100.0 | 0.40 | 11.163 | 0.317 | 21.909 | 0.374 | 57.780 | 0.825 |
| 110.0 | 0.44 | 12.193 | 0.324 | 23.999 | 0.384 | 63.432 | 0.849 |
| 120.0 | 0.48 | 13.220 | 0.328 | 26.086 | 0.388 | 69.116 | 0.856 |
| 130.0 | 0.52 | 14.246 | 0.329 | 28.170 | 0.392 | 74.800 | 0.865 |
| 140.0 | 0.56 | 15.269 | 0.339 | 30.251 | 0.403 | 80.430 | 0.970 |
| 150.0 | 0.60 | 16.292 | 0.350 | 32.332 | 0.413 | 86.056 | 0.974 |
| 160.0 | 0.64 | 17.313 | 0.347 | 34.412 | 0.411 | 91.772 | 0.972 |
| 170.0 | 0.68 | 18.333 | 0.339 | 36.489 | 0.402 | 97.531 | 0.976 |
| 180.0 | 0.72 | 19.350 | 0.354 | 38.565 | 0.420 | 103.101 | 1.008 |
| 190.0 | 0.76 | 20.367 | 0.360 | 40.638 | 0.424 | 108.761 | 1.029 |
| 200.0 | 0.80 | 21.383 | 0.365 | 42.712 | 0.429 | 114.416 | 1.085 |
| 210.0 | 0.84 | 22.396 | 0.369 | 44.782 | 0.432 | 120.077 | 1.030 |
| 220.0 | 0.88 | 23.408 | 0.387 | 46.850 | 0.454 | 125.590 | 1.245 |
| 230.0 | 0.92 | 24.417 | 0.391 | 48.916 | 0.455 | 131.260 | 1.191 |

**Table 2d.** Reduced excess internal energy, $u_{\rm ex}$, reduced excess pressure, $p_{\rm ex}$, and reduced excess inverse isothermal compressibility, $\mu_{\rm ex}$, resulting from molecular dynamics simulations. The standard deviation of the internal energy, $\sigma[u_{\rm ex}]$, and the standard deviation of the pressure, $\sigma[p_{\rm ex}]$, were estimated directly from the fluctuations sampled during the course of the simulation, while the standard deviation of the inverse isothermal compressibility, $\sigma[\mu_{\rm ex}]$, was estimated with the bootstrap resampling technique. **Results for $\boldsymbol{\kappa} = 2.0$**.

| $\Gamma$ | $\Gamma/\Gamma_{\rm m}$ | $u_{\rm ex}$ | $\sigma[u_{\rm ex}] \times 10^3$ | $p_{\rm ex}$ | $\sigma[p_{\rm ex}] \times 10^3$ | $\mu_{\rm ex}$ | $\sigma[\mu_{\rm ex}] \times 10^3$ |
|---|---|---|---|---|---|---|---|
| 45.0 | 0.11 | 2.437 | 0.259 | 5.269 | 0.378 | 13.989 | 0.865 |
| 60.0 | 0.15 | 3.058 | 0.264 | 6.747 | 0.393 | 18.391 | 0.895 |
| 75.0 | 0.19 | 3.665 | 0.279 | 8.199 | 0.420 | 22.644 | 1.017 |
| 90.0 | 0.23 | 4.262 | 0.290 | 9.637 | 0.439 | 26.914 | 1.078 |
| 105.0 | 0.27 | 4.852 | 0.295 | 11.062 | 0.447 | 31.236 | 1.151 |
| 120.0 | 0.30 | 5.438 | 0.298 | 12.481 | 0.454 | 35.551 | 1.138 |
| 135.0 | 0.34 | 6.021 | 0.309 | 13.893 | 0.472 | 39.767 | 1.242 |
| 150.0 | 0.38 | 6.599 | 0.317 | 15.299 | 0.486 | 43.996 | 1.342 |
| 165.0 | 0.42 | 7.176 | 0.327 | 16.702 | 0.502 | 48.201 | 1.410 |
| 180.0 | 0.46 | 7.749 | 0.316 | 18.100 | 0.488 | 52.642 | 1.358 |
| 195.0 | 0.49 | 8.321 | 0.326 | 19.496 | 0.503 | 56.836 | 1.498 |
| 210.0 | 0.53 | 8.891 | 0.328 | 20.887 | 0.506 | 61.122 | 1.505 |
| 225.0 | 0.57 | 9.460 | 0.330 | 22.278 | 0.507 | 65.430 | 1.452 |
| 240.0 | 0.61 | 10.027 | 0.343 | 23.667 | 0.529 | 69.539 | 1.625 |
| 255.0 | 0.64 | 10.593 | 0.344 | 25.053 | 0.529 | 73.839 | 1.581 |
| 270.0 | 0.68 | 11.158 | 0.343 | 26.437 | 0.533 | 78.101 | 1.645 |
| 285.0 | 0.72 | 11.721 | 0.355 | 27.819 | 0.546 | 82.274 | 1.756 |
| 300.0 | 0.76 | 12.283 | 0.350 | 29.199 | 0.539 | 86.629 | 1.671 |
| 315.0 | 0.80 | 12.843 | 0.364 | 30.576 | 0.563 | 90.691 | 1.874 |
| 330.0 | 0.83 | 13.401 | 0.383 | 31.950 | 0.591 | 94.696 | 2.050 |
| 345.0 | 0.87 | 13.959 | 0.372 | 33.324 | 0.572 | 99.155 | 1.901 |
| 360.0 | 0.91 | 14.514 | 0.392 | 34.693 | 0.601 | 103.136 | 2.042 |
| 375.0 | 0.95 | 15.063 | 0.433 | 36.053 | 0.661 | 106.754 | 2.460 |

**Table 2e.** Reduced excess internal energy, $u_{\rm ex}$, reduced excess pressure, $p_{\rm ex}$, and reduced excess inverse isothermal compressibility, $\mu_{\rm ex}$, resulting from molecular dynamics simulations. The standard deviation of the internal energy, $\sigma[u_{\rm ex}]$, and the standard deviation of the pressure, $\sigma[p_{\rm ex}]$, were estimated directly from the fluctuations sampled during the course of the simulation, while the standard deviation of the inverse isothermal compressibility, $\sigma[\mu_{\rm ex}]$, was estimated with the bootstrap resampling technique. **Results for $\boldsymbol{\kappa = 2.5}$.**

| $\Gamma$ | $\Gamma/\Gamma_{\rm m}$ | $u_{\rm ex}$ | $\sigma[u_{\rm ex}] \times 10^3$ | $p_{\rm ex}$ | $\sigma[p_{\rm ex}] \times 10^3$ | $\mu_{\rm ex}$ | $\sigma[\mu_{\rm ex}] \times 10^3$ |
|---|---|---|---|---|---|---|---|
| 80.0 | 0.12 | 1.886 | 0.255 | 4.691 | 0.458 | 13.144 | 1.140 |
| 100.0 | 0.15 | 2.217 | 0.261 | 5.611 | 0.473 | 16.161 | 1.302 |
| 120.0 | 0.18 | 2.540 | 0.274 | 6.515 | 0.502 | 19.014 | 1.468 |
| 140.0 | 0.21 | 2.856 | 0.277 | 7.404 | 0.513 | 21.971 | 1.505 |
| 160.0 | 0.23 | 3.168 | 0.275 | 8.284 | 0.511 | 25.021 | 1.475 |
| 180.0 | 0.26 | 3.477 | 0.293 | 9.157 | 0.548 | 27.708 | 1.694 |
| 200.0 | 0.29 | 3.781 | 0.297 | 10.021 | 0.557 | 30.610 | 2.005 |
| 220.0 | 0.32 | 4.084 | 0.299 | 10.882 | 0.564 | 33.531 | 1.839 |
| 240.0 | 0.35 | 4.384 | 0.303 | 11.737 | 0.575 | 36.390 | 1.910 |
| 260.0 | 0.38 | 4.683 | 0.308 | 12.590 | 0.585 | 39.258 | 1.926 |
| 280.0 | 0.41 | 4.980 | 0.324 | 13.439 | 0.616 | 41.895 | 2.243 |
| 300.0 | 0.44 | 5.274 | 0.316 | 14.282 | 0.603 | 44.970 | 2.121 |
| 320.0 | 0.47 | 5.569 | 0.336 | 15.126 | 0.642 | 47.504 | 2.430 |
| 340.0 | 0.50 | 5.864 | 0.326 | 15.969 | 0.627 | 50.589 | 2.283 |
| 360.0 | 0.53 | 6.156 | 0.327 | 16.807 | 0.627 | 53.520 | 2.288 |
| 380.0 | 0.56 | 6.447 | 0.343 | 17.643 | 0.658 | 56.106 | 2.436 |
| 400.0 | 0.59 | 6.737 | 0.342 | 18.478 | 0.656 | 59.044 | 2.414 |
| 420.0 | 0.62 | 7.026 | 0.336 | 19.311 | 0.647 | 62.060 | 2.520 |
| 440.0 | 0.65 | 7.314 | 0.337 | 20.141 | 0.649 | 64.941 | 2.373 |
| 460.0 | 0.67 | 7.602 | 0.347 | 20.971 | 0.668 | 67.638 | 2.464 |
| 480.0 | 0.70 | 7.889 | 0.354 | 21.800 | 0.683 | 70.375 | 2.773 |
| 500.0 | 0.73 | 8.175 | 0.347 | 22.625 | 0.668 | 73.441 | 2.545 |
| 520.0 | 0.76 | 8.460 | 0.366 | 23.450 | 0.706 | 75.889 | 2.815 |
| 540.0 | 0.79 | 8.745 | 0.364 | 24.274 | 0.703 | 78.815 | 2.812 |
| 560.0 | 0.82 | 9.028 | 0.373 | 25.094 | 0.722 | 81.468 | 3.084 |
| 580.0 | 0.85 | 9.309 | 0.375 | 25.911 | 0.723 | 84.337 | 3.134 |
| 600.0 | 0.88 | 9.590 | 0.372 | 26.727 | 0.722 | 87.222 | 2.859 |
| 620.0 | 0.91 | 9.866 | 0.400 | 27.535 | 0.772 | 89.454 | 3.362 |
| 640.0 | 0.94 | 10.143 | 0.399 | 28.342 | 0.770 | 92.326 | 3.478 |

**Table 2f.** Reduced excess internal energy, $u_{\rm ex}$, reduced excess pressure, $p_{\rm ex}$, and reduced excess inverse isothermal compressibility, $\mu_{\rm ex}$, resulting from molecular dynamics simulations. The standard deviation of the internal energy, $\sigma[u_{\rm ex}]$, and the standard deviation of the pressure, $\sigma[p_{\rm ex}]$, were estimated directly from the fluctuations sampled during the course of the simulation, while the standard deviation of the inverse isothermal compressibility, $\sigma[\mu_{\rm ex}]$, was estimated with the bootstrap resampling technique. **Results for $\boldsymbol{\kappa} = 3.0$**.

| $\Gamma$ | $\Gamma/\Gamma_{\rm m}$ | $u_{\rm ex}$ | $\sigma[u_{\rm ex}] \times 10^3$ | $p_{\rm ex}$ | $\sigma[p_{\rm ex}] \times 10^3$ | $\mu_{\rm ex}$ | $\sigma[\mu_{\rm ex}] \times 10^3$ |
|---|---|---|---|---|---|---|---|
| 150.0 | 0.13 | 1.564 | 0.246 | 4.418 | 0.522 | 13.146 | 1.574 |
| 200.0 | 0.18 | 1.899 | 0.263 | 5.491 | 0.574 | 16.737 | 1.957 |
| 250.0 | 0.22 | 2.220 | 0.277 | 6.529 | 0.614 | 20.309 | 2.126 |
| 300.0 | 0.27 | 2.534 | 0.287 | 7.547 | 0.641 | 23.928 | 2.349 |
| 350.0 | 0.31 | 2.840 | 0.293 | 8.545 | 0.658 | 27.598 | 2.511 |
| 400.0 | 0.35 | 3.140 | 0.300 | 9.529 | 0.679 | 31.153 | 2.646 |
| 450.0 | 0.40 | 3.438 | 0.303 | 10.505 | 0.692 | 34.792 | 2.823 |
| 500.0 | 0.44 | 3.731 | 0.301 | 11.470 | 0.691 | 38.548 | 2.964 |
| 550.0 | 0.49 | 4.022 | 0.319 | 12.430 | 0.731 | 41.797 | 3.090 |
| 600.0 | 0.53 | 4.310 | 0.319 | 13.379 | 0.735 | 45.458 | 3.186 |
| 650.0 | 0.58 | 4.597 | 0.325 | 14.330 | 0.754 | 48.925 | 3.330 |
| 700.0 | 0.62 | 4.882 | 0.330 | 15.272 | 0.765 | 52.467 | 3.415 |
| 750.0 | 0.67 | 5.165 | 0.331 | 16.211 | 0.773 | 56.040 | 3.579 |
| 800.0 | 0.71 | 5.445 | 0.345 | 17.143 | 0.804 | 59.274 | 3.624 |
| 850.0 | 0.75 | 5.726 | 0.345 | 18.077 | 0.804 | 62.935 | 3.985 |
| 900.0 | 0.80 | 6.003 | 0.347 | 19.001 | 0.813 | 66.447 | 3.794 |
| 950.0 | 0.84 | 6.279 | 0.347 | 19.923 | 0.809 | 70.117 | 3.753 |
| 1000.0 | 0.89 | 6.553 | 0.362 | 20.840 | 0.849 | 73.172 | 4.135 |
| 1050.0 | 0.93 | 6.823 | 0.361 | 21.746 | 0.844 | 76.816 | 4.172 |
